# Supplementary material for: Atom Tunneling in the Hydroxylation Process of Taurine/$\alpha$-Ketoglutarate Dioxygenase Identified by Quantum Mechanics/Molecular Mechanics Simulations
Source: arXiv:2009.05441 source file (2020-09-09)
Supplement: Supplementary file 1 [file supporing_info.pdf]

# SUPPORTING INFORMATION TO: Atom Tunneling in the Hydroxylation Process of Taurine/$\alpha$-Ketoglutarate Dioxygenase (TauD) identified by QM/MM Simulations

Sonia Álvarez-Barcia* and Johannes Kästner

*Institute for Theoretical Chemistry, University of Stuttgart, Pfaffenwaldring 55, 70569 Stuttgart, Germany.*

E-mail: alvarez@theochem.uni-stuttgart.de

Phone: +49 (0)711 685-64404. Fax: +49 (0)711 685-64442

## Computational details

### Molecular Dynamics (MD) simulations

The first step was the construction of a model of the enzyme. We started from the crystal structure of *E. coli* TauD with iron, $\alpha$-ketoglutarate and taurine bound to the enzyme (PDB code 1OS7, resolution of 2.50 Å).[1] In the PDB file, 4 monomers can be distinguished; in three of them the taurine is properly linked (i.e. they are closed conformations). We have chosen one of those closed conformations (chain B) to build our model. In order to study the hydroxylation process, we had to modify the structure of the monomer in order to get the quintet [Fe(IV)=O] pre-reactive complex: we added the oxo group to the iron and replaced the $\alpha$-ketoglutarate by succinate.

To properly solvate and equilibrate the enzyme, we carried out MD simulations of the reactant state prior to the QM/MM calculations. The NAMD2 code[2] with the CHARMM22[3–8] force field were used. Parameters for succinate, taurine and the [Fe(IV)=O] complex were defined by homology (see next section). We employed the REDUCE code[9] for adding hydrogen atoms to the enzyme. We solvated the model with a pre-equilibrated box of TIP3P water,[10] in each direction 10 Å wider than the enzyme. $Na^+$ and $Cl^-$ ions (0.15 mol/L) were added to ensure the overall charge neutrality of the model. Both processes were done with VMD (version 1.9.2).[11]

5 MD simulation runs of 4 ns each, starting from random initial velocities were performed at 300 L and 1 bar controlled by a Langevin piston Nóse–Hoover thermostat. A time step of 1 fs was chosen. During the simulations, three steps can be differentiated: a) the solvation process (2000 steps of minimization followed by 50000 steps of MD) where the protein is frozen and the water molecules can spread into the protein; b) MD runs of 50000 steps where the protein atoms were restrained by harmonic potentials with force constants of 5.0, 2.0 and 0.1 kcal $mol^{-1}$ $Å^{-2}$; c) free MD production runs (up to 4 ns). In simulation 1, a slightly different approach was used since only runs of restraints of 5.0 and 2.0 kcal $mol^{-1}$ $Å^{-2}$ were carried out before the free MD.

## QM/MM calculations

We selected 8 snapshots with the shortest (Fe)O–H distances as starting points for the QM/MM optimizations of the reactant states, because these should represent the protein environment in an configuration suitable for the reaction to proceed. We chose a total of 8 snapshots from the 5 simulations. Snapshots 1 and 8 were taken from simulation 5 (at 4.106 and 1.039 ns, respectively); snapshots 2 and 3 from simulation 2 (at 1.956 and 1.985 ns, respectively); snapshots 4 and 6 from simulation 3 (at 3.405 and 0.749 ns, respectively), snapshot 5 from simulation 1 (at 1.558 ns) and snapshot 7 from simulation 4 (at 3.914 ns). The numbering of the snapshots follows the height of the potential energy barrier, see Table 1.

The ChemShell suite was employed for performing the QM/MM calculations.[12–14] It uses an electrostatic embedding, in which the MM charges polarize the QM part. The MM part employed the CHARMM22[3–8] force field in DL_POLY,[15] while the QM calculations were done with TURBOMOLE 7.0.[16]

### Structural/energetic study

For performing the QM/MM calculations, we selected only a part of the model used in the MD simulations. The MM part includes all protein atoms and all residues with at least one atom within a diameter of 20 Å from the Fe atom (5491–5588 atoms depending on the snapshot). Active in the geometry optimizations are all residues with at least one atom within 5 Å from Fe, succinate or taurine (which includes the water molecules that diffused into the inner part of the enzyme). The QM part consists of the truncated amino acids that are directly linked to the Fe ($His_{99}$, $His_{255}$, $Asp_{101}$), as well as a second shell ($Asn_{95}$ and $Arg_{270}$), succinate and taurine. In total, 81 atoms were treated quantum mechanically at the B3LYP/def2-TZVP level[17–19] (see Figure 3). We are considering a neutral QM system with a spin multiplicity of 5.

Initially, geometries of the snapshots selected from the MD simulations were optimized at the B3LYP/def2-SVP level[17–19] using the DL-FIND optimizer.[20] After that, scans along the distance difference d(C-$H_\alpha$)−d($H_\alpha$-O) were computed ($H_\alpha$ being the H abstracted from taurine in the C1 position), by keeping the distance difference constant while minimizing all other degrees of freedom. We started the transition state search by the dimer method[21–24] from the highest energy of the scan. The final geometries were re-optimized at the B3LYP/def2-TZVP level.[17–19]

Minimizations starting from all transitions states after small distortions along the reaction mode were carried out to confirm the structure of the reactant state and its connection to the transition state and to calculate the hydroxyl complex structure as product state.

### Energy comparison

I have changed the position of the table, to be consistent with the manuscript

We have performed some single point calculations with different functionals, taking as reference snapshot 1, in order to test the influence of the DFT method in the barrier (see Table S1).

Table S1: Barrier heights computed with different functionals (with the def2-TZVP basis set) for snapshot 1. The geometry obtained at the B3LYP/def2-TZVP level was used as reference geometry.

| | RS | TS | $\Delta E^{\ddagger}$ |
|---|---|---|---|
| B3LYP | -3780.171516 | -3780.143314 | 17.7 |
| B3LYP (with dispersion) | -3780.342528 | -3780.317119 | 15.9 |
| BHHLYP* | -3780.163414 | -3780.113388 | 31.4 |
| BP86 | -3781.854675 | -3781.822696 | 20.1 |
| M06 | -3780.080007 | -3780.061522 | 11.6 |
| M06-2X* | -3780.516059 | -3780.471434 | 28.0 |
| PBE0 | -3778.696876 | -3778.676569 | 12.7 |
| TPSS | -3781.809024 | -3781.771973 | 23.2 |
| TPSSh | -3781.521584 | -3781.486754 | 21.9 |

* The values with BHHLYP and M06-2X were computed with NWCHEM.[?]

** The selection of the funtionals was done following a paper from Chen *et al.*[?]

### Rate constant calculations

Theoretical reaction rate constants and kinetic isotope effects (KIEs) were computed and compared to experiments. For that purpose, Hessian calculations (two-point finite difference of gradients) of the $H_2C$–Fe=O fragment were carried out in DL-FIND.[20]

Rate constants and KIEs were calculated using transition state theory (TST) taking into account the contribution of atom tunneling by means of the Eckart barrier.[25] The importance of the tunneling can be easily estimated by the crossover temperature $T_c$,[26] which is related to the curvature of the potential at the transition state:

$$T_{\mathrm{c}} = \frac{\hbar\,\Omega}{2\pi k_{\mathrm{B}}} \tag{1}$$

with $\Omega$ being the barrier frequency (the absolute value of the imaginary frequency corresponding to the transition mode) and $k_{\mathrm{B}}$ Boltzmann's constant.

$T_{\mathrm{c}}$ generally indicates the temperature at which tunneling and the thermal mechanism (reaction occurs if the barrier is overcome) have roughly equal importance.[27] Note that $T_{\mathrm{c}}$ is close to room temperature for reactions with $\Omega = 1300$ cm$^{-1}$. Therefore, tunneling is expected to be important at room temperature for higher barrier frequencies.

The doubly deuterated C1-taurine species was used for the KIEs calculations.

### Analysis of the electronic structure during H atom transfer (HAT)

Natural spin densities were calculated by using the TURBOMOLE package[16] (NBO[28] and intrinsic bond orbitals (IBO)[29] approaches were employed) at the B3LYP/def2-TZVP//B3LYP/def2-SVP level for analyzing the course of the reaction. The snapshot with the lowest barrier height (snapshot 1) was chosen for this detailed study.

## Topology and Parameter files for succinate, taurine and the [Fe(IV)=O] complex

### Topology File

In our simulations, we used the CHARMM22 force field, threfore, with the purpose of setting up our system, we have modified the topology file top_all22_prot.inp. 3 new residues were defined in order to simulate the enzyme: the succinate (RESI SUC), the taurine (RESI TAU) and the [Fe(IV)=O] complex (RESI FEO). The patch (PRES FEOX) allows us to change the standard/original charge values for others more appropiate for the TauD enzyme. The charge values for the FEOX patch and the taurine were calculated at the B3LYP/def2-SVP level with the IBOS approach, during the setup of the system, using a QM/MM model similar to the ones employed in the final study.

```
PRES FEOX        -1.68
ATOM 1FE  FE      1.44
ATOM 1OFE OM     -0.55
ATOM 2O1  OC     -0.59
ATOM 2O2  OC     -0.61
ATOM 3NE2 NR2    -0.35
ATOM 4NE2 NR4    -0.35
ATOM 5OD1 OC     -0.67
BOND  1FE 2O2     1FE 3NE2
BOND  1FE 5OD1
BOND  1FE 4NE2    1FE 2O1

RESI FEO          0.89
GROUP
ATOM FE   FE      1.44
ATOM OFE  OM     -0.55
BOND FE  OFE

RESI SUC         -1.68
GROUP
ATOM C4   CT2    -0.28
ATOM HG1  HA      0.09
ATOM HG2  HA      0.09
ATOM C5   CC      0.62
ATOM O4   OC     -0.76
ATOM O3   OC     -0.76
GROUP
```

```
ATOM C3   CT2    -0.28
ATOM HG3  HA      0.09
ATOM HG4  HA      0.09
ATOM C2   CC      0.62
ATOM O1   OC     -0.59
ATOM O2   OC     -0.61
BOND C4 HG1      C4 HG2
BOND C5  C4      C5 O3       C5  O4
BOND C3  C4      C3 HG3      C3 HG4
BOND C2  C3      C2 O1       C2  O2
IMPR C2  C3 O2 O1
IMPR C5  C4 O3 O4
ACCEPTOR O1     C1
ACCEPTOR O2     C1
ACCEPTOR O3     C5
ACCEPTOR O4     C5


RESI TAU          0.00
GROUP
ATOM O1   O      -0.95
ATOM O2   O      -0.98
ATOM O3   O      -0.93
ATOM S    SO      2.13
ATOM C2   CT2    -0.46
ATOM HG1  HA      0.16
ATOM HG2  HA      0.16
```

```
GROUP
ATOM C1   CT2    -0.13
ATOM HE1  HA      0.16
ATOM HE2  HA      0.15
ATOM N1   NH3    -0.34
ATOM HZ1  HC      0.31
ATOM HZ2  HC      0.35
ATOM HZ3  HC      0.37
BOND  N1 HZ1    N1 HZ2    N1 HZ3
BOND  C1 N1     C1 HE1    C1 HE2
BOND  C2 C1     C2 HG1    C2 HG2
BOND  C2 S      S  O1     S  O2    S O3
DONOR HZ1 NZ
DONOR HZ2 NZ
DONOR HZ3 NZ
ACCEPTOR O1 S
ACCEPTOR O2 S
ACCEPTOR O3 S
IC S   C2   *C1  HE1   1.4604 110.4600  119.9100 110.5100  1.1128
IC S   C2   *C1  HE2   1.4604 110.4600 -120.0200 110.5700  1.1123
```

**Parameter File**

In our simulations, we used the CHARMM22 force field, threfore were have added new parameters to the parameter file par_all22_prot.inp in order to fully describe our system. Several parameters for the taurine, the succinate and the Fe=O center were added during the setup of the system (we also modfied three of the original ones, marked with an asterisk). Some of them come from analogous values found them in the original file and other were obtained from QM/MM calculations done during the setup process.

```
BONDS


NR2  FE     65.000     2.1000 *
NR4  CPH1  400.000     1.3800
NR4  CPH2  400.000     1.3200
NR4  FE     65.000     2.1000
OM   FE    250.000     1.6100 *
SO   O     205.000     1.5010
SO   CT2   198.000     1.8180
C    CC    600.000     1.5700
FE   OC    250.000     2.0000


ANGLES


O    SO   O      100.000   112.00
CT2  SO   O      100.000   105.45
HA   CT2  SO      46.100   106.70
CT2  CT2  SO      55.000   110.94
CC   C    CT2     52.000   113.90
C    CC   OC      40.000   118.50
```

```
CC   C    O       80.000   119.47
NR2  FE   OM      50.000   180.00
NR2  FE   OC     100.000    90.93
OC   FE   OM     100.000    93.68
NR2  FE   NR4     50.000    90.00
CC   OC   FE      20.000   135.00
OC   FE   OC     100.000   120.00
CPH2 NR4  CPH1   130.000   104.0000
FE   NR4  CPH1    30.000   133.0000
FE   NR4  CPH2    30.000   123.0000
NR4  CPH1 CPH1   130.000   110.0000
NR4  CPH1 CT2     45.800   120.0000
NR4  CPH1 HR3     25.000   120.00   20.00   2.14000
NR4  CPH2 HR1     25.000   125.00   20.00   2.12000
NR4  CPH2 NR1    130.000   112.5000
NR4  FE   CM      50.000   180.0000
NR4  FE   NPH     50.000   90.0000
NR4  FE   OM      50.000   90.000
NR4  FE   OC     100.000   120.000

DIHEDRALS

O    SO   CT2  CT2        0.2700    3     0.00
O    SO   CT2  HA         0.2000    3     0.00
NR1  CPH2 NR2  FE         0.2000    2   180.00
CPH1 CPH1 NR2  FE         0.2000    2   180.00
HR1  CPH2 NR2  FE         0.2000    2   180.00
```

| | | | | | | |
|---|---|---|---|---|---|---|
| NR2 | FE | OC | CC | 5.2000 | 2 | 0.00 |
| HR3 | CPH1 | NR2 | FE | 0.2000 | 2 | 180.00 |
| CT2 | CC | OC | FE | 0.2000 | 2 | 180.00 |
| CC | OC | FE | OC | 5.2000 | 2 | 180.00 |
| CC | OC | FE | OM | 5.2000 | 2 | 0.00 |
| OC | CC | OC | FE | 5.2000 | 2 | 180.00 |
| CPH2 | NR4 | CPH1 | CPH1 | 14.0000 | 2 | 180.00 |
| CT2 | CPH1 | NR4 | CPH2 | 3.0000 | 2 | 180.00 |
| HR1 | CPH2 | NR4 | CPH1 | 3.0000 | 2 | 180.00 |
| HR3 | CPH1 | NR4 | CPH2 | 3.0000 | 2 | 180.00 |
| NR1 | CPH2 | NR4 | CPH1 | 14.0000 | 2 | 180.00 |
| NR4 | CPH1 | CPH1 | CT2 | 3.0000 | 2 | 180.00 |
| NR4 | CPH1 | CPH1 | CT3 | 3.0000 | 2 | 180.00 |
| NR4 | CPH1 | CPH1 | HR3 | 3.0000 | 2 | 180.00 |
| NR4 | CPH1 | CPH1 | NR1 | 14.0000 | 2 | 180.00 |
| NR4 | CPH1 | CT2 | CT1 | 0.1900 | 3 | 0.00 |
| NR4 | CPH1 | CT2 | CT2 | 0.1900 | 3 | 0.00 |
| NR4 | CPH1 | CT2 | CT3 | 0.1900 | 3 | 0.00 |
| NR4 | CPH1 | CT2 | HA | 0.1900 | 3 | 0.00 |
| NR4 | CPH1 | CT3 | HA | 0.1900 | 3 | 0.00 |
| NR4 | CPH2 | NR1 | CPH1 | 14.0000 | 2 | 180.00 |
| NR4 | CPH2 | NR1 | H | 1.0000 | 2 | 180.00 |
| X | FE | NR4 | X | 0.0500 | 4 | 0.00 |
| NR1 | CPH2 | NR4 | FE | 0.2000 | 2 | 180.00 |
| CPH1 | CPH1 | NR4 | FE | 0.2000 | 2 | 180.00 |
| HR1 | CPH2 | NR4 | FE | 0.2000 | 2 | 180.00 |
| NR4 | FE | OC | CC | 5.2000 | 2 | 180.00 |

```
HR3 CPH1 NR4   FE         0.2000    2   180.00

IMPROPER

C    CC   O    CT2    96.0000         0      0.0000
HR1  NR1  NR4  CPH2    0.5000         0      0.0000
HR1  NR4  NR1  CPH2    0.5000         0      0.0000
HR3  CPH1 NR4  CPH1    0.5000         0      0.0000
HR3  NR4  CPH1 CPH1    0.5000         0      0.0000

NONBONDED

COO    0.000000  -0.070000     2.000000
NR4    0.000000  -0.200000     1.850000
SO     0.000000  -0.450000     2.000000
FE     0.000000  -0.250000     1.090000 *
```

# Results

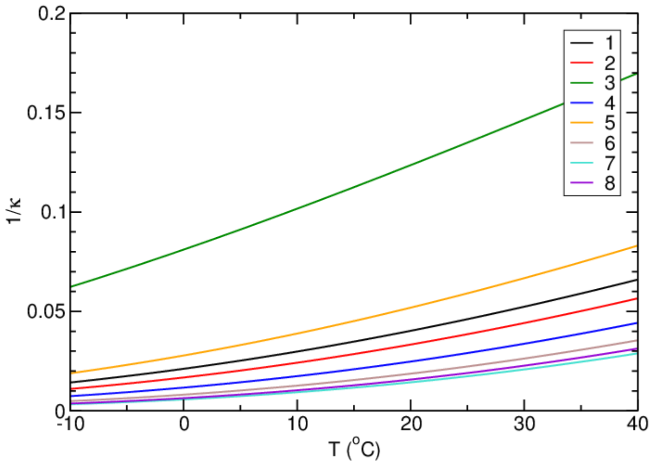


Figure S1: Inverse of $\kappa$ as a function of T (in K) for the 8 snapshots, being $\kappa = k_{\mathrm{Eckart}}/k_{\mathrm{classical}}$; i.e. $\kappa$ represents the increase of the rate constants due to the effect of the tunneling.

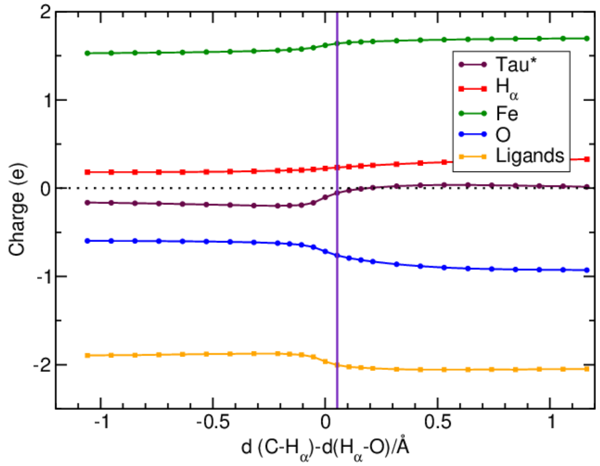


Figure S2: IBO charges along the H-abstraction reaction path for snapshot 1. The distance difference d(C-$H_\alpha$)$-$d($H_\alpha$-O) has been used as reaction coordinate (being $H_\alpha$ the abstracted H from the taurine). The reaction coordinate was computed at the B3LYP/def2-TZVP//B3LYP/def2-SVP level. The vertical violet line shows the position of the TS during the scan.

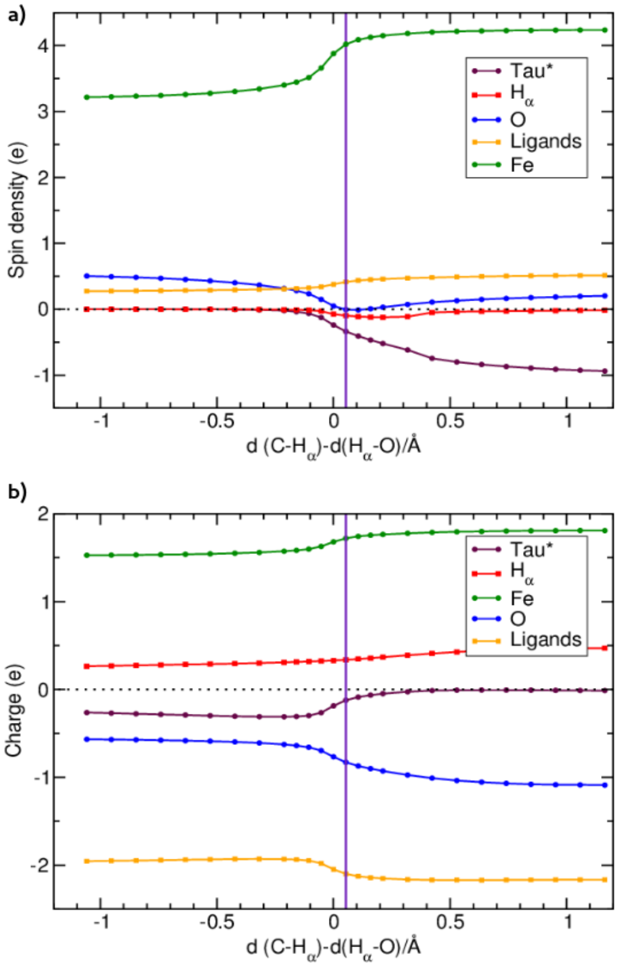


Figure S3: a) NBO spin densities and b) NBO charges along the H-abstraction reaction path for snapshot 1. The distance difference d(C-$H_\alpha$)−d($H_\alpha$-O) has been used as reaction coordinate (being $H_\alpha$ the abstracted H from the taurine). The reaction coordinate was computed at the B3LYP/def2-TZVP//B3LYP/def2-SVP level. The vertical violet line shows the position of the TS during the scan.

# Complete list of authors (manuscript)

**Reference 22**: Baugh L.; Phan I.; Begley D.W.; Matthew C.; Clifton M.C.; Armour B.; Dranow D.M.; Taylor B.M.; Muruthi M.M.; Abendroth J.; Fairman J.W.; Fox III D.; Dieterich S.H.; Staker B.L.; Gardberg A.S.; Choi R.; Hewitt S.N.; Napuli A.J.; Myers J.; Barrett L.K.; Zhang Y.; Ferrell M.; Mundt E.; Thompkins K.; Tran N.; Lyons-Abbott S.; Abramov A.; Sekar A.; Serbzhinskiy D.; Lorimer D.; Buchko G.W.; Stacy R.; Stewart L.J.; Edwards T.E.; Van Voorhis W.C.; and Myler P.J., Tuberculosis **2015**, *95*, 142-148.

**Reference 39**: Sherwood P.; de Vries A.H.; Guest M.F.; Schreckenbach G.; Catlow C.R.A.; French S.A.; Sokol A.A.; Bromley S.T.; Thiel W.; Turner A.J.; Billeter S.; Terstegen F., Thiel S.; Kendrick J.; Rogers S.C.; Casci J.; Watson M.; King F.; Karlsen E.; Sjovoll M.; Fahmi A.; Schafer A.; Lennartz C., Comp. Theor. Chem. **2003**, *632*, 1-28.

# References


(1) O'Brien, J. R.; Schuller, D. J.; Yang, V. S.; Dillard, B. D.; Lanzilotta, W. N. *Biochemistry* **2003**, *42*, 5547–5554.

(2) Phillips, J. C.; Braun, R.; Wang, W.; Gumbart, J.; Tajkhorshid, E.; Villa, E.; Chipot, C.; Skeel, R. D.; Kalé, L.; Schulten, K. *J. Comput. Chem.* **2005**, *26*, 1781–1802.

(3) MacKerell, A. D.; Bashford, D.; Bellott, M.; Dunbrack, R. L.; Evanseck, J. D.; Field, M. J.; Fischer, S.; Gao, J.; Guo, H.; Ha, S. *J. Phys. Chem. B* **1998**, *102*, 3586–3616.

(4) MacKerell, A. D.; Banavali, N. K. *J. Comput. Chem.* **2000**, *21*, 105–120.

(5) Mackerell, A. D.; Feig, M.; Brooks, C. L. *J. Comput. Chem.* **2004**, *25*, 1400–1415.

(6) Feller, S. E.; MacKerell, A. D. *J. Phys. Chem. B* **2000**, *104*, 7510–7515.

(7) Feller, S. E.; Gawrisch, K.; MacKerell, A. D. *J. Am. Chem. Soc.* **2002**, *124*, 318–326.

(8) Foloppe, N.; MacKerell, A. D. *J. Comput. Chem.* **2000**, *21*, 86–104.

(9) Word, J. M.; Lovell, S. C.; Richardson, J. S.; Richardson, D. C. *J. Mol. Biol.* **1999**, *285*, 1735–1747.

(10) Jorgensen, W. L.; Chandrasekhar, J.; Madura, J. D.; Impey, R. W.; Klein, M. L. *J. Chem. Phys.* **1983**, *79*, 926–935.

(11) Humphrey, W.; Dalke, A.; Schulten, K. *J. Mol. Graphics* **1996**, *14*, 27–28.

(12) Sherwood, P. et al. *Comp. Theor. Chem.* **2003**, *632*, 1–28.

(13) Metz, S.; Kästner, J.; Sokol, A. A.; Keal, T. W.; Sherwood, P. *WIREs Comput. Mol. Sci.* **2014**, *4*, 101.

(14) ChemShell, a Computational Chemistry Shell. see http://www.chemshell.org, cited 2017.

(15) Smith, W.; Yong, C.; Rodger, P. *Mol. Simul.* **2002**, *28*, 385–471.

(16) TURBOMOLE V7.0 2015, a development of University of Karlsruhe and Forschungszentrum Karlsruhe GmbH, 1989-2007, TURBOMOLE GmbH, since 2007; available from
`http://www.turbomole.com`. cited 2017.

(17) Becke, A. D. *J. Chem. Phys.* **1993**, *98*, 5648–5652.

(18) Weigend, F.; Ahlrichs, R. *Phys. Chem. Chem. Phys.* **2005**, *7*, 3297–3305.

(19) Weigend, F. *Phys. Chem. Chem. Phys.* **2006**, *8*, 1057–1065.

(20) Kästner, J.; Carr, J. M.; Keal, T. W.; Thiel, W.; Wander, A.; Sherwood, P. *J. Phys. Chem. A* **2009**, *113*, 11856–11865.

(21) Henkelman, G.; Jónsson, H. *J. Chem. Phys.* **1999**, *111*, 7010.

(22) Olsen, R. A.; Kroes, G. J.; Henkelman, G.; Arnaldsson, A.; Jónsson, H. *J. Chem. Phys.* **2004**, *121*, 9776.

(23) Heyden, A.; Bell, A. T.; Keil, F. J. *J. Chem. Phys.* **2005**, *123*, 224101.

(24) Kästner, J.; Sherwood, P. *J. Chem. Phys.* **2008**, *128*, 014106.

(25) Eckart, C. *Phys. Rev.* **1930**, *35*, 1303–1309.

(26) Gillan, M. J. *J. Phys. C: Solid State Physics* **1987**, *20*, 3621–3641.

(27) Kästner, J. *WIREs Comput. Mol. Sci.* **2014**, *4*, 158.

(28) Reed, A. E.; Weinstock, R. B.; Weinhold, F. *J. Chem. Phys.* **1985**, *83*, 735–746.

(29) Knizia, G. *J. Chem. Theory. Comput.* **2013**, *9*, 4834–4843.
